# Supplementary material for: Many Roads Lead to Lithium: Formation Pathways For Lithium-Rich Red Giants
Source: arXiv:2306.03323 source file (2025-01-23)
Supplement: Supplementary file 1 [file appendix.tex]

% In Figure \ref{fig:delta_abundance}, we show the distributions of each available GALAH abundance for our \lirich and \dg samples. The text indicates the average difference and error, where error was calculated as $\textrm{stdev}/\sqrt{N}$ \textbf{(Is it supposed to be N or 2N? I've used both for different plots. Double check with Melissa/Ben.)}
% \begin{figure*}[t!]
%     \centering
%     \includegraphics[width=0.9\textwidth]{compare_abundances_08_22.png}
%     \caption{Distribution of 30 abundances for the \lirich (blue) and \lin (orange) sample. The mean abundance and associated error for both samples is indicated in text with $\mu_R$ and $\mu_P$, respectively.}
%     \label{fig:delta_abundance}
% \end{figure*}

% \begin{figure*}[t!]
%     \centering
%     \includegraphics[width=0.95\textwidth]{apogee_and_galah.png}
%     \caption{}
%     \label{fig:apogee_and_galah}
% \end{figure*}

% \begin{figure*}[t!]
%     \centering
%     \includegraphics[width=0.9\textwidth]{mass_analysis.png}
%     \caption{compared mass vs. tmag, ecl lat, ruwe, numax to figure out why the difference could be happening. also compared teff (from isoclassify and galah and logg. Melissa says galah teff are probably wrong.}
%     \label{fig:mass_analysis}
% \end{figure*}

% \begin{figure*}[h!]
%     \centering
%     \includegraphics[width=0.9\textwidth]{imshow_plot_07_25.png}
%     \caption{all spectra stacked}
%     \label{fig:spectra_stacked}
% \end{figure*}

% \begin{figure*}[t!]
%     \centering
%     \includegraphics[width=0.9\textwidth]{track_-0.25_all.png}
%     \caption{tracks line up i guess?; shows where our samples lie}
%     \label{fig:tracks}
% \end{figure*}

% \begin{figure*}[t!]
%     \centering
%     \includegraphics[width=0.9\textwidth]{placeholder_megan_bedell.png}
%     \caption{\textbf{Megan Bedell Plot: Don't think we need this plot imo.} - \textbf{make similar plot for our sample, but with solar-type stars only!}}
%     \label{}
% \end{figure*}
